# Supplementary material for: The Scallop Theorem and Swimming at the Mesoscale
Source: arXiv:2008.08305 ancillary file (2020-08-19)
Supplement: Supplementary file 1 [file SI_Article.pdf]

# Supplemental Informations on
# "The Scallop Theorem and Swimming at the Mesoscale"

M. Hubert,[1,*] O. Trosman,[1,*] Y. Collard,[2,*] A. Sukhov,[3,*] J. Harting,[3,4] N. Vandewalle,[2] and A.-S. Smith[1,5,†]

[1] *PULS Group, Department of Physics, FAU Erlangen-Nürnberg, IZNF, Erlangen, Germany*
[2] *GRASP, Research unit CESAM, Institute of Physics B5a, Université de Liège, Liège, Belgium*
[3] *Helmholtz Institute Erlangen-Nürnberg for Renewable Energy (IEK-11), Forschungszentrum Jülich, Nürnberg, Germany*
[4] *Deptartment of Chemical and Biological Engineering & Department. of Physics, FAU Erlangen-Nürnberg, Nürnberg, Germany*
[5] *Group for Computational Life Sciences, Ruđer Boskovic Institute, Zagreb, Croatia*

**TABLE OF CONTENTS**

I. Model
- A. The force-based model
- B. The stroke-based model
- C. Relation between stroke-based and force-based approaches
- D. Flow fields

II. Methods
- A. Lattice-Boltzmann simulations
- B. Magneto-capillary swimmers experiments
  1. Description
  2. Parameters
  3. Swimmer velocity

III. Movie

## I. MODEL

### A. The force-based model

Here, we derive the average velocity of the swimmer from the force based approach using the perturbation theory developed in [1]. The equations of motion can be written as

$$\frac{\partial \boldsymbol{x}}{\partial t} = \hat{M}(\boldsymbol{x}) \left[ \boldsymbol{F}(t) + \boldsymbol{G}(\boldsymbol{x}) - \hat{m} \frac{\partial^2 \boldsymbol{x}}{\partial t^2} \right]. \quad (1)$$

The symbol $\boldsymbol{x}$ is a concatenated vector containing the position of beads 1 and 2 such as $\boldsymbol{x} = (\vec{x}_1, \vec{x}_2)$ and $\vec{x}_i = (x_i, y_i, z_i)$. The tensor $\hat{M}$ is the mobility/Oseen tensor and accounts for the hydrodynamic interactions at low Reynolds number. It writes

$$\hat{M} = \begin{pmatrix} \hat{M}_{11} & \hat{M}_{12} \\ \hat{M}_{21} & \hat{M}_{22} \end{pmatrix}, \quad (2)$$

* These authors contributed equally

† Correspondence to: maxime.hubert@fau.de, and ana-suncana.smith@fau.de or asmith@irb.hr

with

$$\hat{M}_{ii} = \frac{1}{6\pi\eta a_i}\hat{1}, \tag{3}$$

$$\hat{M}_{ij} = \frac{1}{8\pi\eta|\vec{x}_i - \vec{x}_j|}\left(\hat{1} + \frac{(\vec{x}_i - \vec{x}_j)\otimes(\vec{x}_i - \vec{x}_j)}{|\vec{x}_i - \vec{x}_j|^2}\right), \tag{4}$$

where $\hat{1}$ is the $3\times 3$ unit tensor, and $\otimes$ denotes the dyadic product. The mobility tensor $\hat{M}$ contains $6\times 6$ elements. The concatenated vectors $\boldsymbol{F}(t)$ and $\boldsymbol{G}(\boldsymbol{x})$, both 6 elements long, write

$$\boldsymbol{F}(t) = \left(\vec{F}_{12}, \vec{F}_{21}\right), \tag{5}$$

$$\vec{F}_{ij} = F\cos(2\pi f t)\,\frac{\vec{x}_i - \vec{x}_j}{|\vec{x}_i - \vec{x}_j|}, \tag{6}$$

and

$$\boldsymbol{G}(\boldsymbol{x}) = \left(\vec{G}_{12}, \vec{G}_{21}\right), \tag{7}$$

$$\vec{G}_{ij} = -k\left(|\vec{x}_i - \vec{x}_j| - L\right)\frac{\vec{x}_i - \vec{x}_j}{|\vec{x}_i - \vec{x}_j|}. \tag{8}$$

Finally, the mass tensor $\hat{m}$ writes

$$\hat{m} = \begin{pmatrix} m_1\hat{1} & 0 \\ 0 & m_2\hat{1} \end{pmatrix}, \tag{9}$$

Equation (1) can be made dimensionless by defining the following quantities: $\vec{x}' = \vec{x}/a$, $\tau = tk/6\pi\eta a$, $\vec{F}' = \vec{F}/F$, $\vec{G}' = \vec{G}/ka$, $\hat{M}' = 6\pi\eta a\hat{M}$ and $\hat{m}' = k\hat{m}/(6\pi\eta a)^2$ with $a$ being the smallest radius. The equations of motion then become

$$\frac{\partial\boldsymbol{x}'}{\partial\tau} = \hat{M}'(\boldsymbol{x}')\left[\epsilon\boldsymbol{F}'(\tau) + \boldsymbol{G}'(\boldsymbol{x}') - \hat{m}'\frac{\partial^2\boldsymbol{x}'}{\partial\tau^2}\right]. \tag{10}$$

The coefficient $\epsilon$ is the normalized amplitude of the external driving force. Our perturbative approach states that having a small parameter $\epsilon$, one can expand the system trajectory $\boldsymbol{x}'(\tau)$ as a series

$$\boldsymbol{x}'(\tau) = \boldsymbol{x}'^{(0)}(\tau) + \epsilon\boldsymbol{x}'^{(1)}(\tau) + \epsilon^2\boldsymbol{x}'^{(2)}(\tau) + \ldots, \tag{11}$$

where $\boldsymbol{x}'^{(0)}$ is the equilibrium configuration of the swimmer for zero driving forces, and the $\boldsymbol{x}'^{(i)}$ represent the displacements around this equilibrium at order $\epsilon^i$. Inserting the above ansatz into the system of differential equations (10), expanding it around small $\epsilon$, and collecting all powers of $\epsilon$, we obtain a new equation

$$\boldsymbol{f}^{(0)}(\tau) + \epsilon\boldsymbol{f}^{(1)}(\tau) + \epsilon^2\boldsymbol{f}^{(2)}(\tau) + ... = 0, \tag{12}$$

where the $\boldsymbol{f}^{(i)}$ are functions of all forces, all positions and all parameters for the order $\epsilon^i$. For $\epsilon \neq 0$, one requires $\boldsymbol{f}^{(i)} = 0\ \forall i$, which gives an infinite set of equations to solve. For example, the zeroth order describes the equilibrium of the system and the first order its oscillation under time-dependent forces. The average swimming velocity is obtained from the second order equation $\boldsymbol{f}^{(2)}(\tau) = 0$ by averaging the result over a period of oscillation of the external driving force [1]. The solution writes

$$\overline{U}^F = \frac{54\pi^2\eta^2F^2\omega^2}{m_1^2m_2^2L^2}\,\frac{a_1^2a_2^2}{a_1+a_2}\,\frac{\left(1-\frac{3a_1}{2L}\right)\left(1-\frac{3a_2}{2L}\right)}{\left(1-\frac{3a_1a_2}{(a_1+a_2)L}\right)}\,\frac{\frac{m_1}{\beta_1}\left(1-\frac{3a_1}{2L}\right) - \frac{m_2}{\beta_2}\left(1-\frac{3a_2}{2L}\right)}{D} \tag{13}$$

$$D = \omega_0^4\left(\frac{\beta_1+\beta_2}{m_1+m_2}\right)^2\left(1-\frac{3a_1a_2}{(a_1+a_2)L}\right)^2 + \omega^2\left(\frac{\beta_1\beta_2}{m_1m_2}\right)^2 - \frac{2\omega_0^2\omega^2}{m_1+m_2}\left(\frac{\beta_2^2}{m_2}\left(1-\frac{3a_1}{2L}\right)^2 + \frac{\beta_1^2}{m_1}\left(1-\frac{3a_2}{2L}\right)^2\right)$$
$$+\,\omega^4\left(\frac{\beta_1^2}{m_1^2} + \frac{\beta_2^2}{m_2^2} + \frac{2\beta_1\beta_2}{m_1m_2}\frac{9a_1a_2}{4L^2}\right) + \omega^2\left(\omega^2-\omega_0^2\right)^2\left(1-\frac{9a_1a_2}{4L^2}\right)^2 \tag{14}$$

### B. The stroke-based model

Contrarily to the *force-based model* discussed in the previous section, the *stroke-based model* assumes that the deformation of the dumbbell is known *a priori* according to the relation

$$\frac{\partial \vec{x}_1}{\partial t} - \frac{\partial \vec{x}_2}{\partial t} = \frac{\partial L}{\partial t}\vec{e}, \tag{15}$$

where $L(t)$ is a known function of time taken here as $L(t) = L + d\sin(\omega t)$, and $\vec{e}$ is the direction set by the axis on the dumbbell. For the theoretical investigation of this model, we start from Eq.(10). Removing the spring by setting $\boldsymbol{G}'(\boldsymbol{x}') = 0$ yields

$$\epsilon \boldsymbol{F}'(\tau) - \hat{m}'\frac{\partial^2 \boldsymbol{x}'}{\partial \tau^2} = \hat{M}'^{-1}(\boldsymbol{x}')\frac{\partial \boldsymbol{x}'}{\partial \tau}. \tag{16}$$

Furthermore, we assume that the swimmer is force free, meaning that the sum of the driving forces over the two beads vanishes, i.e.

$$\vec{F}_{12} + \vec{F}_{21} = 0. \tag{17}$$

Thus, we obtain a system of 4 equations with 4 unknowns being the forces $\vec{F}_{ij}$ and velocities $\partial \vec{x}_i/\partial t$. The solution for the cycle averaged velocity of the center of mass for 2 spheres cannot be obtained analytically without restriction on $a_i/L$. Performing a Taylor expansion of the method up to the second order in $a_i/L$, one obtains

$$\overline{U}^S = \frac{3d^2}{2}\frac{a_1^2 a_2^2}{(a_1+a_2)^3 L^2}\frac{\omega(\theta_2-\theta_1)}{1+\overline{\theta}^2}. \tag{18}$$

### C. Relation between stroke-based and force-based approaches

To relate the two approaches, we calculate the amplitude of oscillation of an one-dimensional asymmetric oscillator. Under the assumption that $a_i/L \ll 1$, the equations of motion are

$$m_1\frac{d^2x_1}{dt^2} + \beta_1\frac{dx_1}{dt} + k(x_1-x_2) = F\cos(\omega t), \tag{19}$$

$$m_2\frac{d^2x_2}{dt^2} + \beta_2\frac{dx_2}{dt} - k(x_1-x_2) = -F\cos(\omega t). \tag{20}$$

Using a Fourier transform, one gets

$$-m_1\tilde{\omega}^2\hat{x}_1 - i\beta_1\tilde{\omega}\hat{x}_1 + k(\hat{x}_1-\hat{x}_2) = \frac{F}{2}\frac{\delta(\tilde{\omega}-\omega)+\delta(\tilde{\omega}-\omega)}{2}, \tag{21}$$

$$-m_2\tilde{\omega}^2\hat{x}_2 - i\beta_2\tilde{\omega}\hat{x}_2 - k(\hat{x}_1-\hat{x}_2) = -\frac{F}{2}\frac{\delta(\tilde{\omega}-\omega)+\delta(\tilde{\omega}-\omega)}{2}, \tag{22}$$

where $\tilde{\omega}$ is the coordinate of the Fourier space. This yields the complex Fourier amplitudes

$$\hat{x}_1(\tilde{\omega}) = \frac{F(i\beta_2+m_2\tilde{\omega})}{ik(\beta_1+\beta_2)+k(m_1+m_2)\tilde{\omega}+\tilde{\omega}(\beta_1-im_1\tilde{\omega})(\beta_2-im_2\tilde{\omega})}\frac{\delta(\tilde{\omega}-\omega)+\delta(\tilde{\omega}-\omega)}{2}, \tag{23}$$

$$\hat{x}_2(\tilde{\omega}) = \frac{F(i\beta_1+m_1\tilde{\omega})}{ik(\beta_1+\beta_2)+k(m_1+m_2)\tilde{\omega}+\tilde{\omega}(\beta_1-im_1\tilde{\omega})(\beta_2-im_2\tilde{\omega})}\frac{\delta(\tilde{\omega}-\omega)+\delta(\tilde{\omega}-\omega)}{2}. \tag{24}$$

Back in real space, the solutions are given by

$$x_1(t) = \left(\hat{x}_1(\omega)e^{-i\omega t} + \left(\hat{x}_1(\omega)e^{-i\omega t}\right)^\dagger\right), \tag{25}$$

$$x_2(t) = \left(\hat{x}_2(\omega)e^{-i\omega t} + \left(\hat{x}_2(\omega)e^{-i\omega t}\right)^\dagger\right), \tag{26}$$

where † corresponds to the complex conjugate. The theory developed by Grosjean *et al.* [2] stipulates that, in Fourier space, the swimming speed is given by

$$\overline{U} \propto \mathrm{Im}\left(\hat{x}_1(\omega)\hat{x}_2^\dagger(\omega)\right) = A_1A_2\sin(\phi_1-\phi_2), \tag{27}$$

which relates the stroke-based and force-based approaches. Given Eqs. (25) and (26), this leads to

$$\mathrm{Im}\left(\hat{x}_1(\omega)\hat{x}_2^\dagger(\omega)\right) = \frac{F^2\omega\left(m_1\beta_2 - m_2\beta_1\right)}{m_1^2 m_2^2\omega^2\left(\left(\omega_0^2-\omega^2\right)+\frac{\beta_1\beta_2}{m_1 m_2}\right)^2 + m_1^2 m_2^2\left(\omega_0^2\frac{\beta_1+\beta_2}{m_1+m_2} - \omega^2\left(\frac{\beta_1}{m_1}+\frac{\beta_2}{m_2}\right)\right)^2}, \tag{28}$$

where we used the relation $\omega_0^2 = k(m_1+m_2)/m_1 m_2$. This last equation corresponds to the swimming speed for the force-based approach (up to a pre-factor containing the geometry of the swimmer). The contributions of each factor in Eq. (27) are the following

$$A_{1,2} = \sqrt{\frac{F\left(\beta_{2,1}^2 + m_{2,1}^2\omega^2\right)}{m_1^2 m_2^2\omega^2\left(\left(\omega_0^2-\omega^2\right)+\frac{\beta_1\beta_2}{m_1 m_2}\right)^2 + m_1^2 m_2^2\left(\omega_0^2\frac{\beta_1+\beta_2}{m_1+m_2} - \omega^2\left(\frac{\beta_1}{m_1}+\frac{\beta_2}{m_2}\right)\right)^2}}, \tag{29}$$

$$\sin\left(\phi_1-\phi_2\right) = \omega\frac{m_1\beta_2 - m_2\beta_1}{\sqrt{\left(\beta_1^2+m_1^2\omega^2\right)\left(\beta_2^2+m_2^2\omega^2\right)}}. \tag{30}$$

As one can see, the origin of the motion, i.e. the asymmetry of coasting time, is carried by the phase shift in this formula. One can cast it as a function of the amplitude of deformation $d$ of the swimmer. Using the Fourier formalism, one has

$$d^2 = \left(\hat{x}_1(\omega)-\hat{x}_2(\omega)\right)\left(\hat{x}_1(\omega)-\hat{x}_2(\omega)\right)^\dagger \tag{31}$$

$$= \frac{\left(\beta_1+\beta_2\right)^2 + \left(m_1+m_2\right)^2\omega^2}{m_1^2 m_2^2\omega^2\left(\left(\omega_0^2-\omega^2\right)+\frac{\beta_1\beta_2}{m_1 m_2}\right)^2 + m_1^2 m_2^2\left(\omega_0^2\frac{\beta_1+\beta_2}{m_1+m_2} - \omega^2\left(\frac{\beta_1}{m_1}+\frac{\beta_2}{m_2}\right)\right)^2}. \tag{32}$$

We have the following relations between $A_1$, $A_2$ and $d$,

$$A_1 = \sqrt{\frac{\left(\beta_1+\beta_2\right)^2 + \left(m_1+m_2\right)^2\omega^2}{\beta_2^2+m_2^2\omega^2}}d, \tag{33}$$

$$A_2 = \sqrt{\frac{\left(\beta_1+\beta_2\right)^2 + \left(m_1+m_2\right)^2\omega^2}{\beta_1^2+m_1^2\omega^2}}d, \tag{34}$$

which yields

$$\mathrm{Im}\left(\hat{x}_1(\omega)\hat{x}_2^\dagger(\omega)\right) = A_1 A_2\sin\left(\phi_1-\phi_2\right) \tag{35}$$

$$= d^2\omega\frac{m_1\beta_2 - m_2\beta_1}{\left(\beta_1+\beta_2\right)^2 + \left(m_1+m_2\right)^2\omega^2}. \tag{36}$$

Up to geometrical pre-factors, this relation corresponds to the result obtained by the Stroke-based approach.

### D. Flow fields

The flow field of the inertial dumbbell can be expressed as

$$\vec{u}_f\left(\vec{x},t\right) = \hat{T}\left(\vec{x}-\vec{x}_1\right).\left(\vec{F}(t) - k\left(\left|\vec{x}_2-\vec{x}_1-L\right|\right) - m_1\frac{d^2\vec{x}_1}{dt^2}\right)$$
$$+ \hat{T}\left(\vec{x}-\vec{x}_2\right).\left(-\vec{F}(t) + k\left(\left|\vec{x}_2-\vec{x}_1-L\right|\right) - m_2\frac{d^2\vec{x}_2}{dt^2}\right) \tag{37}$$

$$= \left(\hat{T}\left(\vec{x}-\vec{x}_1\right) - \hat{T}\left(\vec{x}-\vec{x}_2\right)\right).\left(\vec{F}(t) - k\left(\left|\vec{x}_2-\vec{x}_1-L\right|\right)\right)$$
$$- m_1\hat{T}\left(\vec{x}-\vec{x}_1\right).\frac{d^2\vec{x}_1}{dt^2} - m_2\hat{T}\left(\vec{x}-\vec{x}_2\right).\frac{d^2\vec{x}_2}{dt^2}, \tag{38}$$

where $\hat{T}$ is a second order tensor accounting for the so-called *Oseen tensor* or *Stokeslet*. Assuming that the observation point $\vec{x}$ is such as $|\vec{x}| \gg |\vec{x}_1|, |\vec{x}_2|$, one can use a Taylor expansion on the Oseen tensor and get

$$\hat{T}\left(\vec{x}-\vec{x}_i\right) = \hat{T}\left(\vec{x}\right) - \vec{x}_i.\left(\vec{\nabla}\otimes\hat{T}\left(\vec{x}\right)\right) + \mathcal{O}\left(|\vec{x}_i|^2\right). \tag{39}$$

The second term in the right-hand side of this equation corresponds to the *Stresslet* and is related to the pusher/puller nature of the swimmer. Given this new notation, one can write the instantaneous flow field as

$$\begin{aligned}\vec{u}_f\left(\vec{x},t\right) &= -\hat{T}\left(\vec{x}\right)\left(m_1\frac{d^2\vec{x}_1}{dt^2}+m_2\frac{d^2\vec{x}_2}{dt^2}\right)\\ &+\left(\vec{x}_2-\vec{x}_1\right).\left(\vec{\nabla}\otimes\hat{T}\left(\vec{x}\right)\right).\left(\vec{F}(t)-k\left(|\vec{x}_2-\vec{x}_1-L|\right)\right)\\ &+m_1\vec{x}_1.\left(\vec{\nabla}\otimes\hat{T}\left(\vec{x}\right)\right).\frac{d^2\vec{x}_1}{dt^2}+m_2\vec{x}_2.\left(\vec{\nabla}\otimes\hat{T}\left(\vec{x}\right)\right).\frac{d^2\vec{x}_2}{dt^2}\end{aligned} \tag{40}$$

The first term in the right-hand side accounts for the Stokeslet originating from the inertia of the swimmer. The second term is the usually reported Stresslet for a purely viscous dynamics. The final term is the inertial correction to the viscous Stresslet.

In the linear regime, for a force $|\vec{F}(t)|\sim\cos\left(\omega t\right)$, the position writes $|\vec{x}_i|\sim\cos\left(\omega t+\phi_i\right)$. This implies that once the flow field is averaged over one period $T=2\pi/\omega$, the first order contribution to the flow field vanishes while the second order contributions remain.

## II. METHODS

### A. Lattice Boltzmann simulations

#### 1. *Description*

In order to resolve the hydrodynamic interactions of a two-bead swimmer we employ the lattice Boltzmann (LB) method [3, 4]. It utilizes a discretized version of the Boltzmann equation for the description of the fluid

$$f_i(\vec{x}+\vec{c}_i\Delta t,t+\Delta t)=f_i(\vec{x},t)+\Omega_i(\vec{x},t), \tag{41}$$

which describes the time evolution of a single-particle distribution function $f_i(\vec{x},t)$ at time $t$ and position $\vec{x}$. The vector $\vec{c}_i$ denotes the discrete velocity vector in the $i$th direction of the fluid. We employ a three-dimensional lattice with lattice constant $\Delta x$. The time $t$ is discretized with $\Delta t$-steps. For the sake of simplicity, we present all results in terms of lattice units (l.u.) where $\Delta x$ and $\Delta t$ are set to unity. We use a so-called D3Q19 lattice with $i=1,\ldots,19$ [5]. The left hand side of Eq. (41) is modelled by the free streaming of fluid particles, while their collisions are described by a Bhatnagar-Gross-Krook (BGK) collision operator on the right hand side as [6]

$$\Omega_i(\vec{x},t)=-\frac{f_i(\vec{x},t)-f_i^{\rm eq}(\rho(\vec{x},t),\vec{u}(\vec{x},t))}{\tau}. \tag{42}$$

Here, $f_i^{\rm eq}(\rho(\vec{x},t),\vec{u}(\vec{x},t))$ is a third-order equilibrium distribution function. Macroscopic densities and velocities are defined as $\rho(\vec{x},t)=\rho_0\sum_i f_i(\vec{x},t)$ and $\vec{u}(\vec{x},t)=\sum_i f_i(\vec{x},t)\vec{c}_i/\rho(\vec{x},t)$, respectively ($\rho_0$ is a reference density also set to unity). The parameter $\tau$ is the relaxation time of the fluid that determines the relaxation of $f_i(\vec{x},t)$ towards the equilibrium. The speed of sound $c_{\rm s}=1/\sqrt{3}$ depends on the choice of the lattice geometry and allows one to find both the kinematic $\nu=c_{\rm s}^2(\tau-1/2)$ and the dynamic $\eta=\nu\rho$ fluid viscosities.

The fluid is coupled to a molecular dynamics (MD) algorithm describing the dynamics of suspended rigid particles based on Newton's equations of motion by means of a leap-frog algorithm. The particles are discretized on the lattice and are coupled to the fluid using a modified bounce-back boundary condition [7–9]. When a lattice site $\vec{x}$ is occupied by the surface of a particle, the following equation is applied to its neighboring fluid lattice site $(\vec{x}+\vec{c}_i)$:

$$f_i(\vec{x}+\vec{c}_i,t+1)=f_{\bar{i}}(\vec{x}+\vec{c}_i,t)+\Omega_{\bar{i}}(\vec{x}+\vec{c}_i,t)+C \tag{43}$$

Here, $C$ is a linear function of the local velocity of the particle surface [9] and $\bar{i}$ is defined such that $\vec{c}_i=-\vec{c}_{\bar{i}}$. For conservation of the total momentum of the system, an additional force $\vec{F}_p$ and torque $\vec{D}_p$ are applied on the particle [9] to compensate for the momentum change of the fluid caused by Eq. (43)

$$\vec{F}_{\rm p}=(2f_{\bar{i}}(\vec{x}+\vec{c}_i,t)+C)\vec{c}_{\bar{i}}, \tag{44}$$

$$\vec{D}_{\rm p}=\vec{F}_{\rm p}\times\vec{r}(t), \tag{45}$$

in which $\vec{r}(t)$ is a vector directed from the particle center to the lattice site of reflection. Upon the particle motion the configuration of lattice sites occupied by the particle changes. For newly occupied sites, the fluid on that site is removed and its momentum is added to the particle through a force [9]

$$\vec{F}_{\rm pn} = -\rho(\vec{x}, t)\vec{u}(\vec{x}, t). \tag{46}$$

Vacated lattice sites need to be filled with fluid. We define an average density [9]

$$\bar{\rho}(\vec{x}, t) = \frac{1}{N_{FN}} \sum_{i_{FN}} \rho(\vec{x} + \vec{c}_{i_{FN}}, t), \tag{47}$$

with $N_{FN}$ being the number of neighboring fluid sites with coordinates $\vec{x}_{i_{FN}} = \vec{x} + \vec{c}_{i_{FN}}$. The fluid on the vacated site is then initialized with distribution functions [9]

$$f_i(\vec{x}, t) = \rho_{\rm new} \cdot f_i^{\rm eq}(\vec{u}_{\rm surface}(\vec{x}, t), \rho_{\rm new}(\vec{x}, t)), \tag{48}$$

where $\vec{u}_{\rm surface}(\vec{x}, t)$ is the local velocity of the particle surface and $\rho_{\rm new}(\vec{x}, t)$ corresponds to $\bar{\rho}(\vec{x}, t)$.

#### *2. Parameters*

Two particles with radii $R_1 = 5$ and $R_2 = 8$ and equal densities $\rho_s = 8$ are discretized on the lattice and are surrounded by a fluid with density $\rho_f = 1$ within a simulation box of size $400 \times 160 \times 160$ lattice sites. With a relaxation time $\tau = 1$ and a fluid density $\rho_f = 1$, we obtain a viscosity $\eta = 1/6$ in lattice units. The beads are placed in the center of the box along its longest side. Periodic boundary conditions are used at all edges of the simulation box. The stability of the swimmer is assured by the action of spring forces $F_i(x_i) = -k(x_i - L)$, where $k$ is the spring constant, $x_i$ is the current position of particle $i$ and the equilibrium distance is $L = 28$ lattice sites. We apply external forces $F_i^{\rm ext}(t) = F_{i0}\cos(2\pi f t + \phi_i)$ along the line connecting the particles. To assure the force-free condition required for the self-propulsion of the swimmer, we use $F_{10} = F_{20} = 0.1$ and $\phi_1 = 0$ and $\phi_2 = \pi$.

#### *3. Swimmer velocity*

The velocity of the 2-bead swimmer is calculated via fitting the particle trajectories with the function $A_i\cos(2\pi t/f + B_i) + C_i t + D_i$. The swimmer speed is obtained from $1/2(C_1 + C_2)$ while disregarding the two first periods in the interval $t = [2:20]f^{-1}$.

### B. Magneto-capillary swimmers experiments

A glass container is filled with water and placed in the center of a large triaxial Helmholtz coils system. By injecting electrical current into the coils, spatially uniform magnetic fields can be generated in any direction inside the system. In order to remotely control the interaction between the beads at the water-air interface with magnetic fields, we use two soft ferromagnetic spheres [10]. The beads, made of either martensitic stainless steel (AISI 420) or low-alloy martensitic chrome steel (AISI 52100), have a bulk magnetic susceptibility $\chi \sim 3$ and density $\rho_o = 7830\,\mathrm{kg/m^3}$. Under a magnetic field, these particles behave like an ideal soft magnet, with very little remanence and coercivity. Several bead diameters have been selected : $397\,\mu$m, $500\,\mu$m and $793\,\mu$m. Magnetic dipoles of controllable magnitude and direction can be reversibly induced in the beads using the magnetic fields generated by the Helmholtz coils. The coils parallel to the liquid interface are used to generate a constant and vertical (perpendicular to the interface) magnetic field with amplitude $B_z = 4.9\,$mT or $B_z = 5.6\,$mT. It creates a magnetic repulsion and avoids the contact between the particles, induced by capillary attraction. Oscillating fields are obtained by injecting alternating currents in the two sets of coils perpendicular to the interface, using an amplifier. We consider horizontal field frequencies up to 5 Hz, and amplitudes up to 1 mT. On top of this oscillating field, a constant field is applied with an amplitude of 0.35 mT in order to improve reproducibility and control. The total horizontal field is therefore not oscillating around a zero amplitude. A glass lid coated with a thin metallic conductive layer is placed above the container in order to avoid electrical charges or air displacements that may perturb the motion of the swimmer.

Prior to each experiment, the tank and lid are carefully washed, and the particles and water are replaced. Consistency is essential when filling the tank and placing the particles to avoid variations in the meniscus of the bath and

the contact line of the particles. The bath is lit from below and filmed from the top using a camera equipped with a macro lens. Before each experiment, a noise video is recorded to account for the drift of the beads due to external perturbation (external vibration, air currents, . . . ). For this noise video, the beads are only submitted to the constant magnetic fields without the time-dependent forcing. To measure the position of the particles, they are tracked through a circle Hough transform. The swimming speed is taken as the average distance traveled by the beads over the time of the experiment. This noise is then deduced from the swimmer's speed.

## III. MOVIE

- **SI MOVIE 1** Experimental realization of the inertial dumbbell with beads of $397\,\mu$m and $793\,\mu$m. Parameters are $B_z = 5.60\,$mT,$B_0 = 0.70\,$mT, $\omega = 15.71\,$Hz, $b = 0.35\,$mT.


[1] S. Ziegler *et al*, New J. Phys. **21**, 113017 (2019).
[2] G. Grosjean *et al*, Phys. Rev. E **94**, 021101 (2016).
[3] R. Benzi, S. Succi, and M. Vergassola, Phys. Rep. **222**, 145 (1992).
[4] T. Krüger *et al*, *The Lattice Boltzmann Method*, Graduate Texts in Physics (Springer International Publishing, Cham, 2017).
[5] Y. H. Qian, D. D'Humières, and P. Lallemand, Europhys. Lett. **17**, 479 (1992).
[6] P. L. Bhatnagar, E. P. Gross, and M. Krook, Phys. Rev. **94**, 511 (1954).
[7] A. J. C. Ladd, J. Fluid Mech. **271**, 285 (1994).
[8] A. J. C. Ladd and R. Verberg, J. Stat. Phys. **104**, 1191 (2001).
[9] F. Jansen and J. Harting, Phys. Rev. E **83**, 046707 (2011).
[10] N. Vandewalle *et al*, Phys. Rev. E **85**, 041402 (2012).
